# Supplementary material for: Weak antilocalization in topological insulator Bi$_{2}$Te$_{3}$ microflakes
Source: arXiv:1301.2023 source file (2013-01-10)
Supplement: Supplementary file 1 [file Supplementary_Material.pdf]

# Supplementary Material

for

## “Weak antilocalization in topological insulator $\text{Bi}_2\text{Te}_3$ microflakes”

Shao-Pin Chiu<sup>1</sup> and Juhn-Jong Lin<sup>1,2</sup>

<sup>1</sup>Institute of Physics, National Chiao Tung University, Hsinchu 30010, Taiwan

<sup>2</sup>Department of Electrophysics, National Chiao Tung University, Hsinchu 30010, Taiwan

### I. Determining the effective sample length

We have performed the following experiment to determine the effective sample length  $L_{\text{eff}}$  (hereafter, referred to as  $L$ ) in a four-probe configuration where  $L$  is not significantly greater than the voltage electrode width. Figure s1 shows the sample that we have designed and made to extract a reliable  $L$  value. The conclusion drawn here can be applied to the measurements on other mesoscopic and nanoscale structures, such as the four-probe measurements on single metal and semiconductor nanowires.

We have fabricated micrometer-sized  $\text{Bi}_2\text{Te}_3$  ribbons by the thermal evaporation method combined with the electron-beam lithography technique. Figure s1 shows one long (left) ribbon and one short (right) ribbon prepared simultaneously on a Si substrate capped with a 300 nm thick  $\text{SiO}_2$  layer. The two microribbons are expected to possess similar electrical resistivities. Furthermore, in this test experiment, the two microribbons were grown such that they had resistivities (3–6 m $\Omega$  cm at 300 K) close to that of the BT-24 sample discussed in the paper.

In Fig. s1, the eight large electrodes enclosed by the dotted blocks were made of Ti/Au (10/60 nm) films. Other smaller electrodes and test ribbons were made of 100 nm thick  $\text{Bi}_2\text{Te}_3$ . The left long ribbon allows us to accurately determine the sample resistivity from the standard four-probe measurement, by using a and d as the current electrodes and b and c as the voltage electrodes. We obtained a resistivity of 5.9 m $\Omega$  cm at 300 K. Then we measured the right microribbon by using both the four-probe configurations with electrodes (e,f,g,h) and electrodes (f,g,h,i). These measurements allowed us to determine the resistance  $R$  of the segments (f,g) and (g,h), respectively. Because the resistivity  $\rho$ , the width  $w$  and the thickness  $t$  of the microribbon were known, we could then calculate the effective sample lengths of the two short segments (f,g) and (g,h) from  $L = Rwt/\rho$ . We had found that the effective sample lengths thus determined agreed to within 10% to the closest distance  $L_{\text{min}}$  between the two “wide” voltage electrodes. It should be noted that we had prepared and measured four sets of long and short microribbons and found that this conclusion held true in all sets. (The

widths of e, f, g, and h electrodes were varied from set to set.)

In short, we found that the effective sample length  $L$  always fell in the range  $(1.0-1.1) \times L_{\min}$ , being independent of the width of the voltage electrodes. This uncertainty in  $L$  could transfer to an error bar in our measured sheet resistance  $R_{\square}$  by an amount of at most 10%.

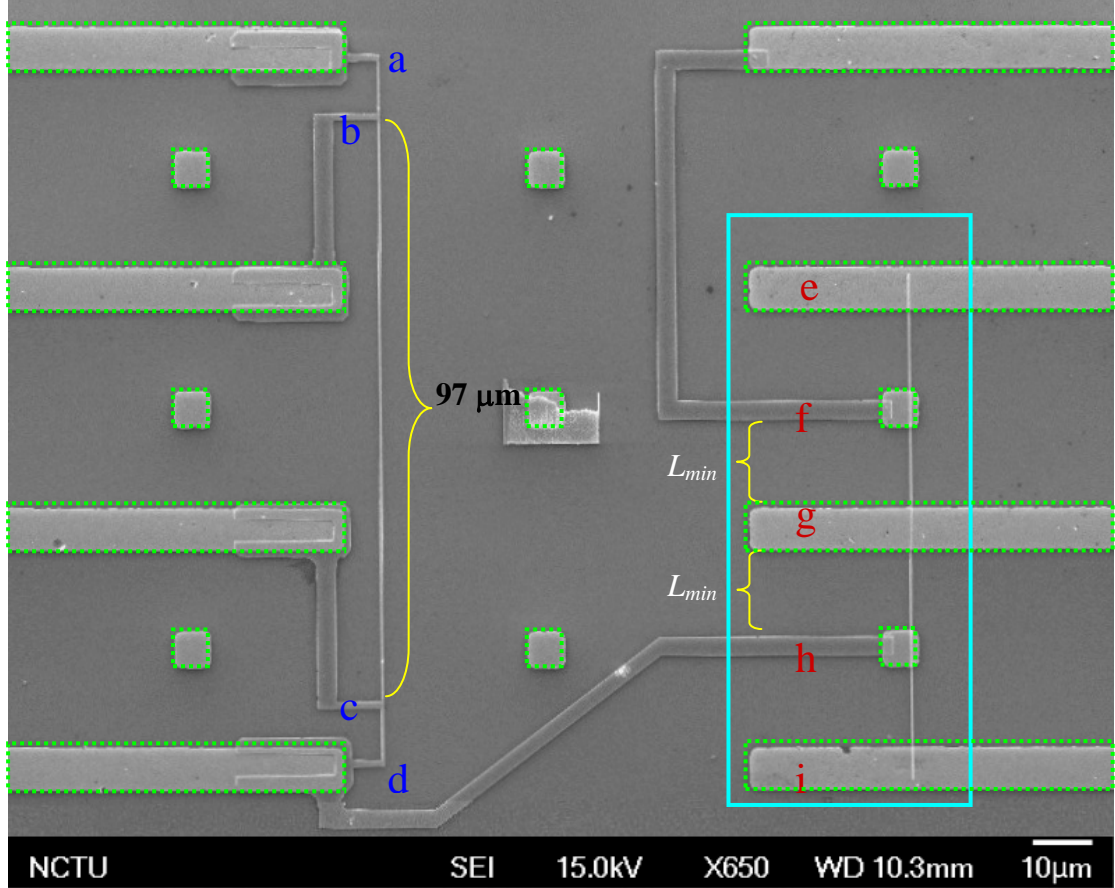

**Fig. s1** A set of micrometer-sized  $\text{Bi}_2\text{Te}_3$  ribbons for extracting the effective sample length  $L$  in a four-probe configuration where  $L$  is not significantly greater than the voltage electrode width.

## II. Variation of resistance with backgate voltage

We have measured the resistance  $R$  as a function of backgate voltage  $V_{\text{BG}}$  of the BT-23 microflake at several temperatures. The BT-23 was grown simultaneously with the BT-15 and BT-24 samples discussed in the main text. The BT-23 microflake was chosen because it possessed dimensions (70 nm thickness, 1  $\mu\text{m}$  width, and 1.2  $\mu\text{m}$  length) and electrical properties (5.5  $\text{m}\Omega\text{ cm}$  at 300 K and 1.2  $\text{m}\Omega\text{ cm}$  at 4 K) similar to those of the BT-24 microflake discussed in the paper.

The applied  $V_{\text{BG}}$  was varied from  $-60$  to  $+60$  V, and our results are plotted in Fig. s2(a). We

expect the Fermi level  $E_F$  associated with the bottom surface to be tunable by  $V_{BG}$ . Figure s2(a) shows that, at every temperature, the  $R(V_{BG})$  curve reveals a maximum at a characteristic  $V_{BG}^*$  value. This characteristic  $V_{BG}^*$  value corresponds to the situation where the Fermi level was aligned to the Dirac point. [Taking the  $T = 2$  K curve as an example, we found  $V_{BG}^* \approx +7$  V, as schematically illustrated by the blue dashed line in Fig. s2(b).] That is, the appearance of a maximum in the  $R(V_{BG})$  curve is suggestive of the existence of topological surface states. Note that above  $V_{BG}^*$ , our measured  $R$  value only progressively decreased with further increase in  $V_{BG}$  up to our largest  $+60$  V. In other words, if our applied  $V_{BG}$  were sufficiently large so that  $E_F$  had been shifted to pass through the conduction band minimum [schematically indicated by the red dashed line in Fig. s2(b)], an electron accumulation layer would form and a sharp drop in the  $R(V_{BG})$  curve should happen at a certain  $V_{BG} > V_{BG}^*$ . This was clearly not the case. Therefore, up to our largest  $V_{BG} = +60$  V, the Fermi level still fell below the conduction band minimum, and no accumulation layer was formed in the device under study. According to current theoretical understanding, it is thus most plausible to ascribe our observed two coherent conduction channels to the bottom topological surface states and the bulk states.

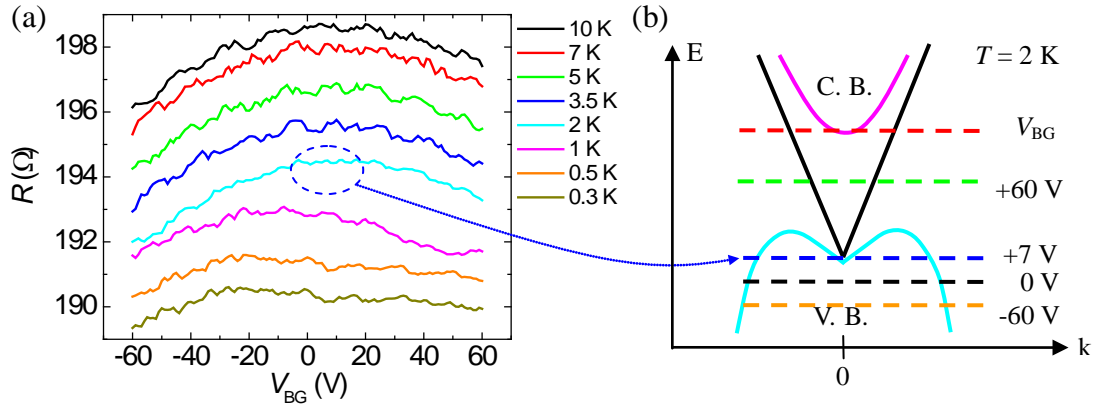

**Fig. s2** (a)  $R(V_{BG})$  curves of the BT-23 microflake at several temperatures, as indicated. The curves are offset for clarity. (b) A schematic band diagram for the topological insulator  $\text{Bi}_2\text{Te}_3$ . The straight dashed lines mark the positions of the Fermi level at different applied  $V_{BG}$  values for the  $T = 2$  K case.
